# Supplementary material for: Benchmarks and Explanations for Deep Learning Estimates of X-ray Galaxy Cluster Masses
Source: arXiv:2303.00005 source file (2023-07-25)
Supplement: Supplementary file 1 [file 8_appendix.tex]

\appendix

\rev{
\section{Locality Tests for Data Leakage}\label{apx:locality}
The problem is this

To solve it we did this

These are the results}
